# Supplementary material for: Multi-Model 3D Registration: Finding Multiple Moving Objects in Cluttered Point Clouds
Source: arXiv:2402.10865 source file (2024-02-16)
Supplement: Supplementary file 1 [file appendix.tex]

%!TEX root = ../main.tex

% \begin{restatable}{lemma}[Consistency]{consistency}

\begin{theorem}[Hoeffding's Inequality]
\label{thm:hoeffding}
Let $x_1, ..., x_n$ be i.i.d random variables such as $|x_i| \leq a$ almost surely. Then, we have the following inequality, with probability $1-\delta$,
\begin{align}\label{eqn:hoeffding_bound}
\left |\frac 1 n \sum_{i=1}^n x_i - \E[x_i] \right | \leq a \sqrt{\frac 2 n \log{\frac 2 \delta}}.
\end{align}
\end{theorem}
\textbf{Remark:} If we have $k$ such sets of i.i.d. random variables variables $\{x_{j,1}, \dots, x_{j, n}\}_{j=1}^k$ all having the same distribution with mean $0$, then for each of these sets, eq.\eqref{eqn:hoeffding_bound} is not satisfied with probability at most $\delta$. In the worst case, the chance that eq.~\eqref{eqn:hoeffding_bound}   fails to hold \emph{simultaneously} for these is given by $1 - (1 - \delta)^k < 1 - (1 - k \delta )  = k \delta$ when $\delta \ll 1$. Hence, by replacing $\delta$ with $\delta/k$ in \Cref{thm:hoeffding} and taking a union bound, we see that with probability at least $1-k \cdot (\delta/k) = 1-\delta$,
\begin{align}\label{eqn:hoeffding_bound}
\red{\sum_{j=1}^k \left |\frac 1 n \sum_{i=1}^n x_{j, i} \right | \leq ak \sqrt{\frac 2 n \log{\frac {2k} \delta}}.}
\end{align}
We will often use this version of the inequality below. \new{SK: Cite this.}
\begin{theorem}[Trace Lower Bound] %   of the trace of  positive definite matrix product
\label{thm:tr_lb}
Let $\MA$ be a positive definite matrix. Then, 
\begin{align*}
Tr(\MA \MB) \geq \lambda_{\min}(\MA) Tr(\MB)
\end{align*}
where $\lambda_{\min}(A)$ is the smallest eigenvalue value of $\MA$.
\end{theorem}

\begin{lemma}[Consistency]
\label{lem:HornRepeat}
Let $\{ (\va_i, \vb_i) \}_{i=1}^m \subset \!\Real{3}\! \times\! \Real{3}$ be $m$ samples satisfying 
$\vb_i = \MR \va_i + \vt + \vepsilon_i$ where $\vepsilon_i$ is drawn uniformly from $[-\sigma, \sigma]^3$, $\MR \in \SOthree$ is a rotation matrix and $\vt \in \Real{3}$ is a translation vector. Let $\Sigma \!=\! \frac 1 m \sum_i \va'_i (\va'_i)\tran$, where $\va_i' := \va_i - \frac 1 n \sum_{i=1}^n \va_i$.
Then, with probability $1\!-\!2 \delta$, Horn's method returns $(\hat \MR, \hat \vt)$ such that 
\begin{align*}
\|\hat \MR - \MR\|_F^2 \leq \frac {18 B \sigma}{\lambda_{min}(\MSigma)}\sqrt{\frac{2}{m} \log \frac {18} \delta }
\end{align*}
and,
\begin{align*}
\| \hat \vt - \vt \|_2^2 \leq  36 B \sigma  \sqrt{\frac{2}{m} \log \frac {18} \delta } +
\frac{12}{m} \sigma^2 \log \frac {6} \delta 
\end{align*}
\end{lemma}

% \begin{lemma}[Consistency]
% \label{lem:HornRepeat}
% Let $\{ (\va_i, \vb_i) \}_{i=1}^m \subset \Real{3} \times \Real{3}$ be $m$ samples satisfying 
% $\vb_i = \MR \va_i + \vt + \vepsilon_i$ where $\vepsilon_i$ is drawn uniformly from $[-\sigma, \sigma]^3$, $\MR \in \SOthree$ is a rotation matrix and $\vt \in \Real{3}$ is a translation vector. Let $\Sigma = \frac 1 m \sum_i \va_i \va_i\tran$.
% Then, with probability $1-2\delta$, Horn's method returns $(\hat \MR, \hat \vt)$ such that 
% \begin{align*}
% \|\hat \MR - \MR\|_F^2 \leq \frac {18 B \sigma}{\lambda_{min}(\MSigma)}\sqrt{\frac{2}{m} \log \frac {\textcolor{red}{18}} \delta }
% \end{align*}
% and,
% \begin{align*}
% \| \hat \vt - \vt \|_2^2 \leq  36 B \sigma  \sqrt{\frac{2}{m} \log \frac {\textcolor{red}{18}} \delta } +
% \frac{12}{m} \sigma^2 \log \frac {\textcolor{red}{6}} \delta 
% \end{align*}
% \end{lemma}
% \end{restatable}

\emph{Proof:}
We first define $\va_i'$ and $\vb_i'$, which are centered versions of our data, and do the same for the noise:
\begin{equation}
\va_i' = \va_i - \frac 1 n \sum_{i=1}^n \va_i,  \;\;
\vb_i' = \vb_i - \frac 1 n \sum_{i=1}^n \vb_i, \;\;
\vepsilon_i' = \vepsilon_i - \frac 1 n \sum_{i=1}^n \vepsilon_i
\end{equation}

\noindent
% Let $\hat{\MR}$ be our estimate of $\MR$. 
After centering the data (which amounts to algebraically eliminating the translation from the problem, see~\cite{Horn87josa}), Horn's method looks for a rotation $\MX\!\in\!\SOthree$ that maximizes the following objective:
% over $\MX\!\in\!\SOthree$: % being an rotation matrix:
\begin{align}
&\langle \MX,  \frac 1 m \sum^m_{i=1} \va'_i (\vb'_i)\tran \rangle \\
&= \langle \MX, \frac 1 m \sum^m_{i=1} \va'_i (\MR \va'_i +\vepsilon'_i)\tran\rangle \\
&= \langle \MX, \frac 1 m \sum^m_{i=1} (\va'_i (\va'_i)\tran \MR\tran + \va'_i (\vepsilon')_i\tran) \rangle \\ 
&= \langle \MX, \frac 1 m \sum^m_{i=1}   \va'_i (\va'_i)\tran \MR\tran \rangle + \langle \MX, \frac 1 m \sum^m_{i=1} \va'_i (\vepsilon'_i)\tran \rangle \\
&= \frac 1 m \sum^m_{i=1} \langle \MX,  \va'_i (\va'_i)\tran \MR\tran \rangle + \langle \MX, \frac 1 m \sum^m_{i=1} \va'_i (\vepsilon'_i)\tran \rangle \\
&:= f(\MX) + h(\MX) 
\end{align}
% \red{An application of Hoeffding's inequality tells us that the centered random variables $\vepsilon'_i$ for $i \in [m]$ are still bounded -- 
% since $\MX_{i,j} \leq 1$, $\|\va_i\| \leq B$  and $\vepsilon_{i,j} \leq \sigma$, 
% we have $\vepsilon'_{i, j} = \vepsilon_{i, j} - \frac{1}{m} \sum_{i=1}^{m} \vepsilon_{i, j} \leq \sigma + \sigma \sqrt{\frac{2}{m} \log{\frac{\textcolor{red}{18}}{\delta}}}$} simultaneously, for all $i \in [m], j \in [3]$ with probability at least $1-\delta$. Each entry of the second term can be bounded simultaneously with probability $1-\delta$ using Hoeffding's inequality again and a union bound over the number of dimensions. 
Since, for $i\in [ m ], j\in [ 3 ]$, the $j$-th entry of $\vepsilon_{i}$, namely $\vepsilon_{i,j}$, satisfies $|\vepsilon_{i,j}| \leq \sigma$, we have $|\vepsilon'_{i, j}| = |\vepsilon_{i, j} - \frac{1}{m} \sum_{i=1}^{m} \vepsilon_{i, j}| \leq 2 \sigma$. Then, since $|\MX_{j, k}| \leq 1$, $\|\va_i\| \leq B$, each entry of the second term can be bounded simultaneously with probability $1-\delta$ using Hoeffding's inequality and a union bound over the number of dimensions, as follows.  
For any rotation matrix $\MX$, we have
\begin{align} \label{eqn:h_bound}
|h(\MX)| 
&= \left | \sum_{j, k \in [3]} \MX_{j, k} \left (\frac 1 m \sum^m_{i=1} \va_i (\vepsilon'_i)\tran \right)_{j, k} \right | \\
% &= \left | \left \frac 1 m \sum^m_{i=1} \sum_{j, k \in [3]} \MX_{j, k} \va_{i, j} \vepsilon'_{i, k} \right | \\
&\text{\color{gray} (applying the triangle inequality)}\\
&\leq \sum_{j, k \in [3]} \left | \frac 1 m \sum^m_{i=1} \MX_{j, k} \left (\va_i (\vepsilon'_i)\tran \right)_{j, k} \right | \\
&\text{\color{gray} (applying Hoeffding's inequality in Theorem \ref{thm:hoeffding})}\\
% &\leq 3 \cdot (B \sigma) \left(1 + \sqrt{\frac{2}{m} \log \frac{\textcolor{red}{18}} \delta }\right) \cdot \sqrt{\frac{2}{m} \log \frac 2 \delta}\\
% & \leq 3^2 \cdot  B (2 \sigma)  \sqrt{\frac{2}{m} \log \frac {\textcolor{red}{2 \cdot 3^2}} \delta } \\
&\leq 18 B \sigma  \sqrt{\frac{2}{m} \log \frac {18} {\delta} }
% &\leq 3B \sigma (\frac{1}{\sqrt m} \log{\frac 1 \delta} + \sqrt{\frac{2}{m} \log{\frac{1}{\delta}}})
\end{align}
Let 
% $\MR = \max_{\MX \in SO(3)} f(\MX)$ (in other words, $\MR = \MR$) and 
$\hat \MR = \max_{\MX \in SO(3)} f(\MX) + h(\MX)$ and recall that the ground-truth rotation $\MR$ satisfies $\MR = \max_{\MX \in SO(3)} f(\MX)$ (this is due to the fact that a noiseless registration problem recovers the ground truth exactly). Then, eq.~\eqref{eqn:h_bound} implies
\begin{align}
&\quad f(\MR)  + 18 B \sigma  \sqrt{\frac{2}{m} \log \frac {18} \delta } \\
&\quad \color{gray} (\text{using }\MR = \textstyle\max_{\MX \in SO(3)} f(\MX) ) \\
&\geq f(\hat \MR)  + 18 B \sigma  \sqrt{\frac{2}{m} \log \frac {18} \delta } \\
&\quad \color{gray}  (\text{using eq.~}\eqref{eqn:h_bound}) \\
&\geq f(\hat \MR) + h(\hat \MR) \\
&\quad \color{gray} (\text{using }\hat \MR = \max_{\MX \in SO(3)} f(\MX) + h(\MX)) \\
&\geq f(\MR) + h(\MR). 
\end{align}
Subtracting $f(\MR) + h(\hat \MR)$, 
another application of \eqref{eqn:h_bound} gives
\begin{align}
& f(\MR)  +18  B \sigma  \sqrt{\frac{2}{m} \log \frac {18} \delta } - f(\MR) -h(\hat \MR)\\
&\quad \geq f(\hat \MR) + h(\hat \MR) - f(\MR) -h(\hat \MR) \\
& 18 B \sigma  \sqrt{\frac{2}{m} \log \frac {18} \delta } -h(\hat \MR) \geq f(\hat \MR)  - f(\MR) \\
& 36 B \sigma  \sqrt{\frac{2}{m} \log \frac {18} \delta }  \geq f(\hat \MR)  - f(\MR)
\end{align}
and
\begin{align}
& f(\hat \MR) + h(\hat \MR) - f(\MR) -h(\hat \MR) \\
&\quad \color{gray} (\text{using }\hat \MR = \max_{\MX \in SO(3)} f(\MX) + h(\MX)) \\
&\quad \geq f(\MR) + h(\MR) - f(\MR) -h(\hat \MR) \\
& f(\hat \MR) - f(\MR) \geq h(\MR) -h(\hat \MR) \\
&\quad \color{gray}  (\text{using eq.~}\eqref{eqn:h_bound}) \\
& f(\hat \MR) - f(\MR) \geq - 36 B \sigma  \sqrt{\frac{2}{m} \log \frac{18}{\delta} }
\end{align}
Then, we have
\begin{align}\label{eq:function_closeness}
|f(\hat \MR) - f(\MR)| \leq 36B \sigma  \sqrt{\frac{2}{m} \log \frac {18} \delta }
\end{align}
In what follows, we will need the following observations:
\begin{align} \label{eq:ip_to_norm}
\frac 1 2 f(\hat{\MR}) &= 
\frac 1 m \sum_i (\|\hat{\MR} \va'_i\|_2^2 + \|\MR \va'_i\|_2^2 -\|\hat{\MR} \va'_i - \MR \va'_i \|_2^2)\\
&= \frac 1 m \sum_i (\|\va'_i\|_2^2 + \|\va'_i\|_2^2 -\|\hat{\MR} \va'_i - \MR \va'_i \|_2^2) \\
&= \frac 1 m \sum_i (2 \|\va'_i\|_2^2  -\|\hat{\MR} \va'_i - \MR \va'_i \|_2^2).
\end{align}
Also, 
\begin{align}
\frac 1 2 f(\MR) &= \frac 1 m \sum_i 2 \|\va'_i\|_2^2
\end{align}

We now show that \eqref{eq:function_closeness} implies closeness in parameters. 
% As a first step, we show that $\frac 1 m \sum_i \|\hat \MR \va_i - \MR \va_i\|^2$ is bounded. 
% Recall that $\hat \MR$ minimizes $\frac 1 m \sum_i \|\MX \va_i - \MR \va_i - \vepsilon_i\|^2$ and $\MR$ minimizes $\frac 1 m \sum_i \|\MX \va_i - \MR \va_i\|^2$.
Substituting eq.~\eqref{eq:ip_to_norm} into \eqref{eq:function_closeness}, we see,  
\begin{align}
&\frac 1 2 |f(\hat \MR) - f(\MR)| \\
&= \left| \frac 1 m \sum_i (2 \|\va'_i\|^2  -\|\hat \MR \va'_i - \MR \va'_i \|_2^2 - 2 \|\va'_i\|^2) \right| \\
&= \left| \frac 1 m \sum_i   \|\hat \MR \va'_i - \MR \va'_i \|_2^2  \right| \\
% &\leq \frac 1 m \sum_i  \left| \|\hat \MR \va_i - \MR \va_i \|_2^2  \right| \\
&= \frac 1 m \sum_i  \|\hat \MR \va'_i - \MR \va'_i \|_2^2 \\
&\quad \color{gray}  (\text{using eq.}~\eqref{eq:function_closeness}) \\
&\leq 18 B \sigma  \sqrt{\frac{2}{m} \log \frac {18} \delta }.
% \frac 1 m |\sum_i  (Tr(\MR \va_i \va_i\tran {(\MR)}\tran) -  Tr(\MR \va_i \va_i\tran  {(\hat \MR)}\tran))| &< 6 \frac{B \sigma}{\sqrt m} \log{\frac 1 \delta} \\
% \frac 1 m |\sum_i (2Tr(\MR \va_i \va_i\tran {(\MR)}\tran) - 2Tr(\MR \va_i \va_i\tran  {(\hat \MR)}\tran) -  & \\
% (\|\MR \va_i\|^2 + \|\MR \va_i\|^2) + (\|\hat \MR \va_i\|^2 + \|\MR \va_i\|^2))| &< 12 \frac{B \sigma}{\sqrt m} \log{\frac 1 \delta} \\
% &24 B \sigma  \sqrt{\frac{2}{m} \log \frac {\textcolor{red}{18}} \delta } \\
% &> \frac 1 m \left |\sum_i (\| \MR \va_i - \MR \va_i\|^2 - \|\hat \MR \va_i - \MR \va_i\|^2)\right |\\
% &= \frac 1 m \sum_i \|\hat \MR \va_i - \MR \va_i\|^2. 
\end{align}
To show that $\hat \MR$ and $\MR$ are close, we will now further lower bound $\frac 1 m \sum_i \|\hat \MR \va'_i - \MR \va'_i\|^2$ in terms of $\| \hat \MR - \MR\|_F$. In what follows, let $\MSigma = \frac 1 m \sum_i \va'_i (\va'_i)\tran$ and $\lambda_{\min}(\MSigma)$ be the smallest eigenvalue of $\MSigma$:
% \textcolor{red}{Note: Please reference the relevant facts we use to lower bound these quantities in terms of $\lambda_{min}$. We need a small section that lists out these facts.}
%
\begin{align}
&\quad~\frac 1 m \sum_i \|\hat \MR \va'_i - \MR \va'_i\|^2 \\
&= \frac 1 m \sum_i (\va'_i)\tran (\hat \MR - \MR)\tran (\hat \MR - \MR) \va'_i \\
&= \frac 1 m \sum_i Tr((\hat \MR - \MR)\tran (\hat \MR - \MR) \va'_i (\va'_i)\tran) \\
&=   Tr((\hat \MR - \MR)\tran (\hat \MR - \MR)   \frac 1 m \sum_i \va'_i (\va'_i)\tran) \\
&=   Tr((\hat \MR - \MR)\tran (\hat \MR - \MR)   \MSigma) \\
&\quad \color{gray} \text{(using Theorem \ref{thm:tr_lb})} \\
&\geq \lambda_{min}(\MSigma) Tr((\hat \MR - \MR)\tran (\hat \MR - \MR)) \\
&\geq \lambda_{min}(\MSigma) \|\hat \MR - \MR\|_F^2.
\end{align}

Thus, we have 
$
\|\hat \MR - \MR\|_F^2 \leq \frac {18} {\lambda_{min}(\MSigma)} B \sigma  \sqrt{\frac{2}{m} \log \frac {18} \delta }
$. 

Let $\hat t= \frac 1 m \sum_i(\vb_i - \hat \MR \va_i)$ be our estimate of the translation $t$. We now show that $\hat \vt$ is close to $\vt$. 
\begin{align}
\hat \vt &= \frac 1 m \sum_i(\vb_i - \hat \MR \va_i) \\
&= \frac 1 m \sum_i(\MR \va_i + \vt + \vepsilon_i - \hat \MR \va_i) \\
&= \vt + \frac 1 m \sum_i(\MR - \hat \MR) \va_i + \frac 1 m \sum_i \vepsilon_i.
\end{align}

The difference between the estimate $\hat \vt$ and the ground truth $\vt$ can be upper bounded as follows,
\begin{align}
&\quad \|\hat \vt-\vt\|^2 \\
% &= \|\frac 1 m \sum_i(\vb_i - \hat \MR \va_i) - \vt\|^2 \\
% &= \|\frac 1 m \sum_i(\MR \va_i + \vt + \vepsilon_i - \hat \MR \va_i) - \vt\|^2 \\
&= \left\|\frac 1 m \sum_i(\MR - \hat \MR) \va_i + \frac 1 m \sum_i \vepsilon_i \right\|^2 \\
&\leq 2\left\|\frac 1 m \sum_i(\MR - \hat \MR) \va_i\right\|^2 + 2\left\|\frac 1 m \sum_i \vepsilon_i \right\|^2 \\
&\leq \frac 2 m \sum_i \left\|(\MR - \hat \MR) \va_i\right\|^2 + 2\left\|\frac 1 m \sum_i \vepsilon_i \right\|^2 \\
% &\leq 24 \frac{B \sigma}{\sqrt m} \log{\frac 1 \delta} + 2\|D \frac{\sigma}{\sqrt{m}} \log{\frac {1} {\delta}} \|^2 \\
&\leq  36 B \sigma  \sqrt{\frac{2}{m} \log \frac {18} \delta } +
\red{\frac{12}{m} \sigma^2 \log \frac {6} \delta }
% \frac{6\sigma^2}{m} \log^2{\frac {1} {\delta}}
\end{align}

% \begin{align}
% &\quad \|\hat \vt-\vt\| \\
% % &= \|\frac 1 m \sum_i(\vb_i - \hat \MR \va_i) - \vt\| \\
% % &= \|\frac 1 m \sum_i(\MR \va_i + \vt + \vepsilon_i - \hat \MR \va_i) - \vt\| \\
% &= \|\frac 1 m \sum_i(\MR - \hat \MR) \va_i + \frac 1 m \sum_i \vepsilon_i \| \\
% &\leq \|\frac 1 m \sum_i(\MR - \hat \MR) \va_i\| + \|\frac 1 m \sum_i \vepsilon_i \| \\
% &\leq \frac 1 m \sum_i \|(\MR - \hat \MR) \va_i\|^2 + \frac 1 m \sum_i \| \vepsilon_i \| \\
% &\leq 24 \frac{B \sigma}{\sqrt m} \log{\frac 1 \delta} + 2\|D \frac{\sigma}{\sqrt{m}} \log{\frac {1} {\delta}} \|^2 \\
% &\leq 24 \frac{B \sigma}{\sqrt m} \log{\frac 1 \delta} + D' \frac{\sigma^2}{m} \log^2{\frac {1} {\delta}}
% \end{align}
% \textcolor{red}{SK: I don't think we need the last part so I commented it out.}
% Lastly, we have, for any $i$, the error of the estimate given by the Horn's method

% \begin{align}
% &\quad \|\vb_i - \hat \MR \va_i -\hat \vt \| \\
% &= \|\MR \va_i + \vt - \hat \MR \va_i - \hat \vt  \| \\
% &= \|\MR \va_i + \vt + \vepsilon_i - \hat \MR \va_i - \hat \vt  \| \\
% &\leq \|(\MR - \hat \MR) \va_i\| + \|\vt  - \hat \vt  \|  + \| \vepsilon_i \|\\
% &\leq (\frac {12}{\lambda_{min}(\MSigma)} \frac{B \sigma}{\sqrt m} \log{\frac 1 \delta})^{\frac 1 2} B \\
% &\quad +(24 \frac{B \sigma}{\sqrt m} \log{\frac 1 \delta} + D' \frac{\sigma^2}{m} \log^2{\frac {1} {\delta}})^{\frac 1 2} + \sqrt{3} \sigma
% \end{align}
